# Supplementary material for: Self-supervised Point Cloud Prediction Using 3D Spatio-temporal Convolutional Networks
Source: arXiv:2110.04076 source file (2021-10-18)
Supplement: Supplementary file 1 [file supplementary.pdf]

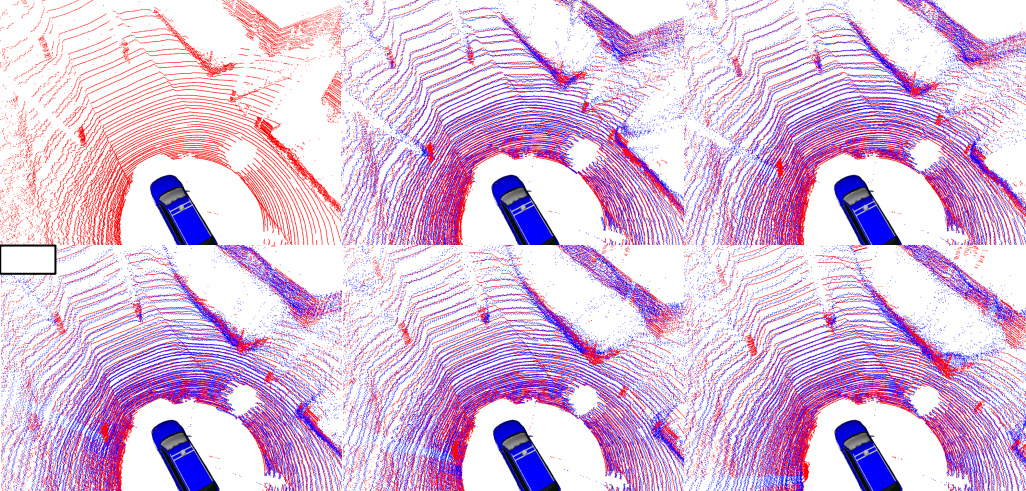

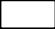

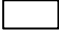

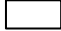

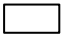

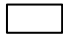

|  |  |  |
|--|--|--|
|  |  |  |
|  |  |  |
