# Supplementary material for: Self-supervised Point Cloud Prediction Using 3D Spatio-temporal Convolutional Networks
Source: arXiv:2110.04076 source file (2021-10-18)

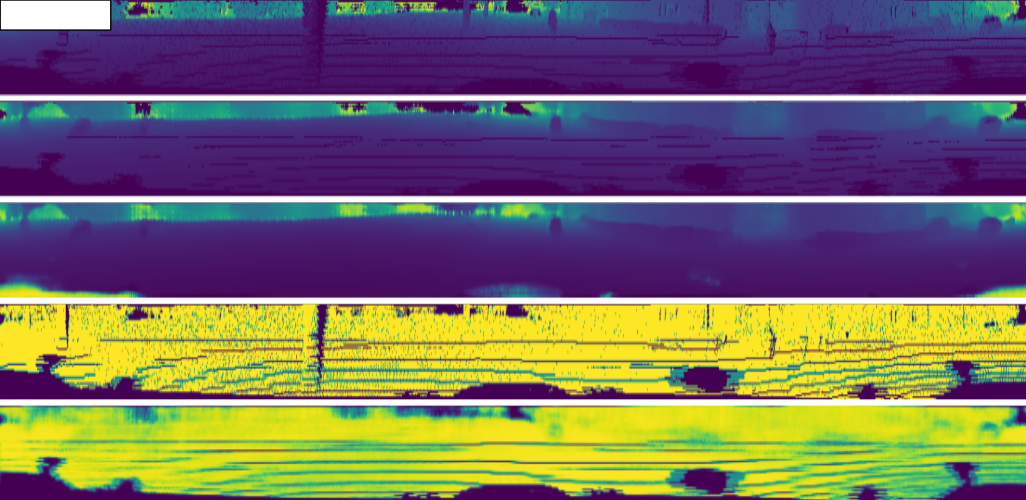

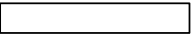

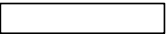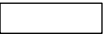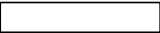

Supplement: Supplementary file 2 [file supplementary_range_image.pdf]
